# Supplementary material for: Structural results for the Tree Builder Random Walk
Source: arXiv:2311.18734 source file (2024-12-06)
Supplement: Supplementary file 1 [file appendix.tex]

\section{Generalized Law of Iterated Logarithm}
\begin{theorem}[Kolmogorov]\label{thm:lil}Let $\{X_k\}_k$ be a sequence of mean zero independent random variables with $EX_k^2 <\infty$ for all $k$. Suppose that 
\begin{equation*}
    B_n := \sum_{k=1}^n EX^2_k \stackrel{n\to \infty}{\longrightarrow} \infty
\end{equation*}
and exists $M_k \ge |X_k|$ such that 
$$
M_k = o\left( \sqrt{B_k/\log\log B_k}\right).
$$
Then,
$$
\liminf_{n\to \infty}\frac{\sum_{k=1}^n X_k}{\sqrt{2B_n\log \log B_n}} = \limsup_{n\to \infty}\frac{\left|\sum_{k=1}^n X_k\right|}{\sqrt{2B_n\log \log B_n}} = 1, \text{a.s}
$$
\end{theorem}
